# Supplementary material for: Spin Excitation Spectra of Anisotropic Spin-$1/2$ Triangular Lattice Heisenberg Antiferromagnets
Source: arXiv:2201.12121 source file (2022-11-23)
Supplement: Supplementary file 1 [file Appendix.pdf]

# *Supplementary material*

# Spin Excitation Spectra of Anisotropic Spin-$1/2$ Triangular Lattice Heisenberg Antiferromagnets


Runze Chi,[1,2,*] Yang Liu,[1,2,*] Yuan Wan,[1,3] Hai-Jun Liao,[1,3,†] and T. Xiang[1,2,4,‡]

[1]*Beijing National Laboratory for Condensed Matter Physics and Institute of Physics, Chinese Academy of Sciences, Beijing 100190, China.*
[2]*School of Physical Sciences, University of Chinese Academy of Sciences, Beijing 100049, China.*
[3]*Songshan Lake Materials Laboratory, Dongguan, Guangdong 523808, China.*
[4]*Beijing Academy of Quantum Information Sciences, Beijing, China.*


## I. TENSOR NETWORK REPRESENTATION OF THE GROUND STATE

To simulate the magnetic excitations of $\mathrm{Ba_3CoSb_2O_9}$, we need to calculate the zero-temperature dynamical spectral function

$$\begin{aligned} & S^{\alpha\beta}(\boldsymbol{k},\omega) \\ = & \langle 0|S^{\alpha}_{-\boldsymbol{k}}\delta(\omega - H + E_0)S^{\beta}_{\boldsymbol{k}}|0\rangle \\ = & \sum_m \langle 0|S^{\alpha}_{-\boldsymbol{k}}|m\rangle\langle m|S^{\beta}_{\boldsymbol{k}}|0\rangle\delta(\omega - E_m + E_0), \end{aligned} \quad \text{(Q1)}$$

where $H$ is the Hamiltonian, $\alpha, \beta = x, y, z$ are the spin components. $|m\rangle$ represents either the ground state if $m = 0$ or an excited states if $m \neq 0$. $E_m$ is the corresponding energy eigenvalue.

In our calculation, the ground state $|0\rangle \equiv |\Psi(A)\rangle$ is represented by an infinite projected entangled-pair state (iPEPS) on a deformed square lattice, which is obtained from the original triangular lattice by grouping three sites on a triangle into one site

$\Psi(A) =$ 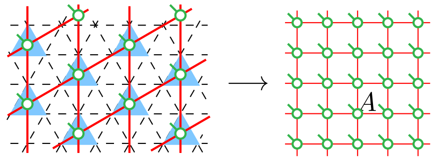 (Q2)



Local tensor $A$ is assumed to be translation invariant. It contains three physical spins and is determined by variationally minimizing the ground state energy. This minimization is implemented by making use of the automatic differentiation [R1]. An accurate determination of local tensor $A$ is crucial to the calculation of excitation spectra.

Once obtaining the optimized local tensors, we evaluate the expectation value of a physical observable by contracting the tensor-network states using the corner-transfer-matrix renormalization group (CTMRG). The result such obtained depends on both the bond dimension of the iPEPS, $D$, and the boundary bond dimension of CTMRG, $\chi$. To obtain a better estimation of the expectation value, we extrapolate the results first to the limit $1/\chi \to 0$ for a given $D$ and then to the limit $1/D \to 0$.

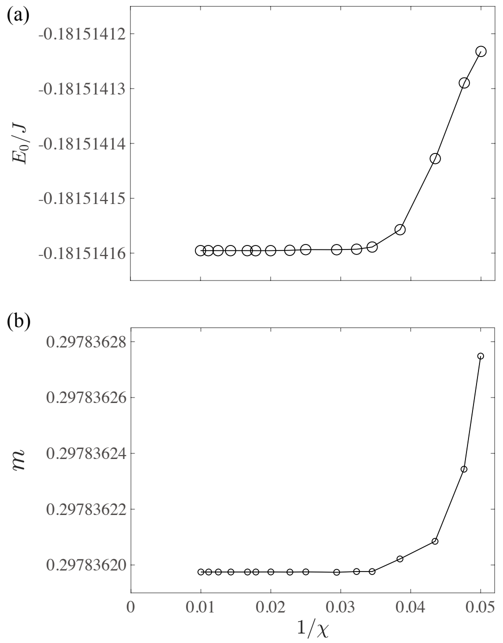



FIG. S1. The ground state energy $E_0$ (a) and the magnetization $m$ (b) as functions of $1/\chi$ for the isotropic TLAFHM ($\Delta = 1.0$). The bond dimension of iPEPS $D = 4$.

Figure S1 shows how the ground state energy $E_0$ and the magnetization $m$ converge with $1/\chi$ for the isotropic Heisenberg model obtained with the $D = 4$ iPEPS. In general, the CTMRG results should converge when $\chi$ becomes sufficiently greater than $D^2$. This is indeed what we find from Fig. S1. By extrapolating the results to the limit $1/\chi \to 0$, we obtain the values of the ground state energy $E_0(D)$ and the magnetization $m(D)$ at a given $D$.

After obtaining the extrapolation values in the limit $\chi \to \infty$, we extrapolate $E_0$ and $m$ with respect to $1/D$. Fig. S2 shows how the ground state energy and the magnetization converge with $1/D$ for both isotropic and anisotropic triangular-lattice antiferromagnetic Heisenberg models (TLAFHM). By fitting the iPEPS data with a power-law formula $E_0(D) = e_0 + aD^{-\alpha}$, we find that $E_0(\Delta = 0.95) = -0.1811J$ and $E_0(\Delta = 1.0) = -0.1840J$. For the isotropic TLAFHM with $\Delta = 1.0$, our result agrees with the DMRG result $-0.1837(7)J$ [R2] as well as the Coupled Cluster result


* These authors contributed equally to this work
† navyphysics@iphy.ac.cn
‡ txiang@iphy.ac.cn

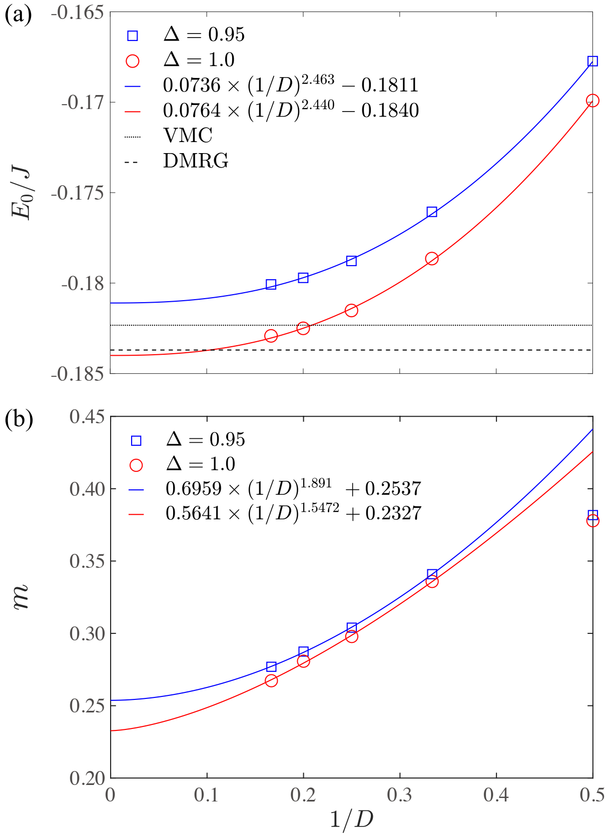


FIG. S2. Inverse bond-dimension dependences of (a) the ground state energy $E_0$ and (b) the magnetization $m$ for the anisotropic (blue square, $\Delta = 0.95$) and isotropic (red circle, $\Delta = 1.0$) TLAFHM. The ground state energies obtained from DMRG [R2] and VMC [R4] are shown in panel (a) for comparison.

$-0.1838J$ [R3], and is lower than the variational Monte Carlo (VMC) result $-0.18233(3)J$ [R4] and the Green function Monte Carlo result $-0.18193(3)$ [R5]. It suggests that $\Psi(A)$ presents an accurate representation of the ground state of TLAFHM.

Similarly, we find that the magnetization also shows a power-law dependence on $D$, $m(D) = m_0 + bD^{-\beta}$. By fitting, we find that the extrapolated magnetization in the limit $1/D \to 0$ is $m_0 = 0.2537$ and $m_0 = 0.2327$ for the model with $\Delta = 0.95$ and 1.0, respectively. The magnetization $m_0$ of the anisotropic TLAFHM ($\Delta = 0.95$) is slightly greater than the isotropic one ($\Delta = 1.0$) because the easy-plane anisotropy favors more strongly the coplanar 120° ordered ground state.

## II. CALCULATION OF THE EXCITATION SPECTRUM

In the framework of tensor-network states, an excited state $|m\rangle$ is described by a tangent vector that is perpendicular to the ground state under the single-mode approximation [R6]. More specifically, $|m\rangle$ is obtained in two steps. First, we replace the local tensor $A$ at site $\boldsymbol{r}$ in $|\Psi(A)\rangle$ with a new tensor $B$ and denote it as $|\Phi_{\boldsymbol{r}}(B)\rangle$,

$$\Phi_{\boldsymbol{r}}(B) = \qquad \text{(Q3)}$$

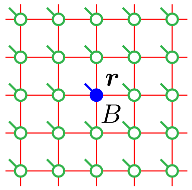


Second, we boost $|\Phi_{\boldsymbol{r}}(B)\rangle$ into a momentum eigenstate:

$$|\Phi_{\boldsymbol{k}}(B)\rangle = \sum_{\boldsymbol{r}} e^{i\boldsymbol{k}\cdot\boldsymbol{r}} |\Phi_{\boldsymbol{r}}(B)\rangle. \qquad \text{(Q4)}$$

This single-mode approximated wave function was first introduced in the framework of matrix product states (MPS) by Ostlund and Rommer in one dimension [R7, R8]. It was extended to PEPS in two dimensions by Vanderstraeten *et. al.* [R9].

The excited states such defined are the momentum eigenstates. They should be orthogonal to the ground state. This requires that $|\Phi_{\boldsymbol{r}}(B)\rangle$ be a vector in the tangent space of the ground state, satisfying the constraint

$$\langle \Phi_{\boldsymbol{r}}(B^\dagger)|\Psi(A)\rangle = 0. \qquad \text{(Q5)}$$

Furthermore, it is simple to show that $|\Phi_{\mathbf{k}}(B)\rangle$ is invariant under the gauge transformation [R9]

$$B \to B + e^{i\boldsymbol{k}} AX - XA, \qquad \text{(Q6)}$$

where $X$ is an arbitrary $D \times D$ bond matrix. This implies that $|\Phi_{\mathbf{k}}(B)\rangle$ is a null tensor network state if $B$ takes the value

$$B_X = e^{i\boldsymbol{k}} AX - XA. \qquad \text{(Q7)}$$

Thus to determine the physically allowed $B$-tensors in the tangent space, one should exclude the tensors in the subspace spanned by all linearly independent $B_X$-tensors. This step is important to ensure the stability of the effective norm matrix $N^{\text{eff}}$, defined by Eq. (Q8), in solving the generalized eigenequation (Q14). As a PEPS has two perpendicular bond directions, there are $2D^2 + 1$ linearly independent $B$-tensors that should be excluded.

To find the excited states, we start from all physically allowed and orthogonal $B$-tensors, denoted as $\tilde{B}_m$, in the tangent space of the ground state. The norm matrix is defined by the wave function overlap between different tangent vectors

$$N^{\text{eff}}_{mn} = \langle \Phi_{\boldsymbol{k}}(\tilde{B}^\dagger_m)|\Phi_{\boldsymbol{k}}(\tilde{B}_n)\rangle. \qquad \text{(Q8)}$$

The corresponding Hamiltonian matrix is

$$H^{\text{eff}}_{mn} = \langle \Phi_{\boldsymbol{k}}(\tilde{B}^\dagger_m)|H|\Phi_{\boldsymbol{k}}(\tilde{B}_n)\rangle. \qquad \text{(Q9)}$$

Since $N^{\text{eff}}_{mn}$ and $H^{\text{eff}}_{mn}$ are linear functions of local tensor $\tilde{B}^\dagger_m$ and $\tilde{B}_n$, they can also be written as

$$N^{\text{eff}}_{mn} = \tilde{B}^\dagger_m \mathbb{N}_{\boldsymbol{k}} \tilde{B}_n, \quad H^{\text{eff}}_{mn} = \tilde{B}^\dagger_m \mathbb{H}_{\boldsymbol{k}} \tilde{B}_n, \qquad \text{(Q10)}$$

where $\mathbb{N}_{\boldsymbol{k}}$ and $\mathbb{H}_{\boldsymbol{k}}$ are $M \times M$ matrices.

As $\mathbb{N}_{\boldsymbol{k}}$ and $\mathbb{H}_{\boldsymbol{k}}$ do not explicitly depend on $\tilde{B}$-tensors, the above expression suggests that both $\mathbb{N}_{\boldsymbol{k}}\tilde{B}_n$ and $\mathbb{H}_{\boldsymbol{k}}\tilde{B}_n$ can be determined by simply taking the derivative of the diagonal term of the norm matrix $N^{\text{eff}}_{nn}$ and effective Hamiltonian $H^{\text{eff}}_{nn}$ with respect to $\tilde{B}^\dagger_n$, respectively,

$$\left(\mathbb{N}_{\boldsymbol{k}}\tilde{B}_n\right) = \frac{\partial}{\partial\tilde{B}^\dagger_n}\left(\tilde{B}^\dagger_n\mathbb{N}_{\boldsymbol{k}}\tilde{B}_n\right), \tag{Q11}$$

$$\left(\mathbb{H}_{\boldsymbol{k}}\tilde{B}_n\right) = \frac{\partial}{\partial\tilde{B}^\dagger_n}\left(\tilde{B}^\dagger_n\mathbb{H}_{\boldsymbol{k}}\tilde{B}_n\right). \tag{Q12}$$

The above derivatives, as discussed in Ref. [R11], can be evaluated by utilizing the automatic differentiation [R1]. From these derivatives, we can obtain all the matrix elements of $N^{\text{eff}}_{mn}$ and $H^{\text{eff}}_{mn}$, namely,

$$N^{\text{eff}}_{mn} = \tilde{B}^\dagger_m\left(\mathbb{N}_{\boldsymbol{k}}\tilde{B}_n\right), \quad H^{\text{eff}}_{mn} = \tilde{B}^\dagger_m\left(\mathbb{H}_{\boldsymbol{k}}\tilde{B}_n\right). \tag{Q13}$$

By solving the following generalized eigen-equation,

$$\sum_n H^{\text{eff}}_{mn}v_{np} = \sum_n E_p N^{\text{eff}}_{mn}v_{np}. \tag{Q14}$$

we obtain the $B$-tensor of the $m$th excited state

$$B_m = \sum_n \tilde{B}_n v_{nm}, \tag{Q15}$$

and the corresponding excitation energy $E_m$. Finally, we can use these results to calculate the zero-temperature dynamical spectral function (Q1).

The main computational cost is to evaluate the derivative of $H^{\text{eff}}_{nn}$ for each independent excited basis state, which scales as $O(D^{12})$ [R1, R11]. For each momentum point $\boldsymbol{k}$, the total computational cost scales as $O(\mathcal{N}\times D^{12})$, where $\mathcal{N}\sim dD^4 - 2D^2 - 1$ is the total number of excited basis states and $d$ is the physical bond dimension.

## III. SUM RULE OF THE DYNAMICAL SPECTRAL FUNCTION

After obtaining the wave functions of the excitation states, we can calculate the dynamical spectral function using the formula

$$S^{\alpha\alpha}(\boldsymbol{k},\omega) = \sum_m w^\alpha_{\boldsymbol{k}}(m)\delta(\omega - E_m + E_0), \tag{Q16}$$

where

$$w^\alpha_{\boldsymbol{k}}(m) = \left|\langle\Phi_{\boldsymbol{k}}(B^\dagger_m)\,|S^\alpha_{\boldsymbol{k}}|\,\Psi(A)\rangle\right|^2 \tag{Q17}$$

is the spectral weight, and the delta function is expanded by a Lorentzian broadening factor $\eta$, which mimics the finite temperature broadening effect for spectra function.

If the single-spin excited states $|\Phi_{\boldsymbol{k}}(B_m)\rangle$ are complete, it is expected that the dynamical spectral function should satisfy the following sum rule

$$\sum_{m,\alpha} w^\alpha_{\boldsymbol{k}}(m) = \sum_\alpha\left[\langle 0|S^\alpha_{-\boldsymbol{k}}S^\alpha_{\boldsymbol{k}}|0\rangle - |\langle 0|S^\alpha_{\boldsymbol{k}}|0\rangle|^2\right]. \tag{Q18}$$

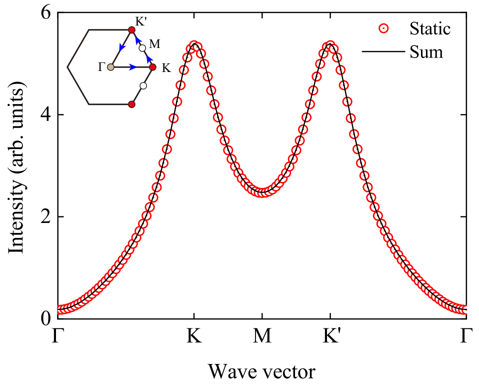


FIG. S3. Verification of the sum rule for the dynamical spectral function. Comparison of the total spectral weights (black curve) with the static spin structure factor (red circles) along the momentum path $\Gamma - \text{K} - \text{M} - \text{K}' - \Gamma$.

The right hand side of this equation is the static spin structure factor, which is determined purely by the ground state wave function $|\Psi(A)\rangle$.

Fig. S3 compares the total spectral weights with the static spin structure factor along the momentum path $\Gamma - \text{K} - \text{M} - \text{K}' - \Gamma$. Clearly, the sum rule is satisfied.

## IV. BASIS NUMBER DEPENDENCE OF SPIN EXCITATION SPECTRA

The solution of the generalized eigenequation (Q14) may become unstable if the norm matrix is ill-conditioned. This instability can be removed if we can eliminate all redundant gauge degrees of freedom, including the null modes, in $|\Phi_k(B)\rangle$ and reduce the numerical error in the normal matrix $N^{\text{eff}}$ to a sufficiently low level. For the $D=2$ case, we indeed

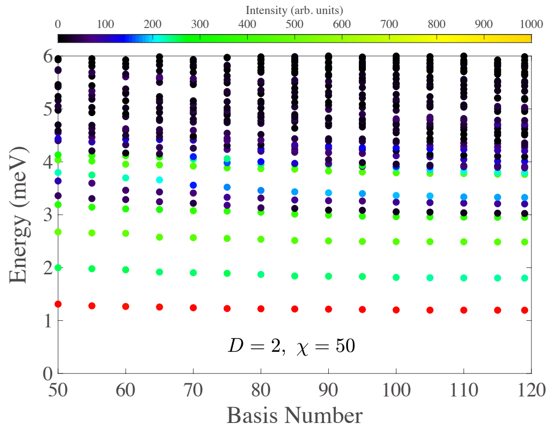


FIG. S4. Dependence of the spin excitation spectra on the basis number of the norm matrix for the anisotropic TLAFHM ($\Delta = 0.95$) at the $M$ point obtained with the $D = 2$ PEPS wave function. $\chi = 50$ is used in the CTMRG contraction. The color denotes the spectral weight.

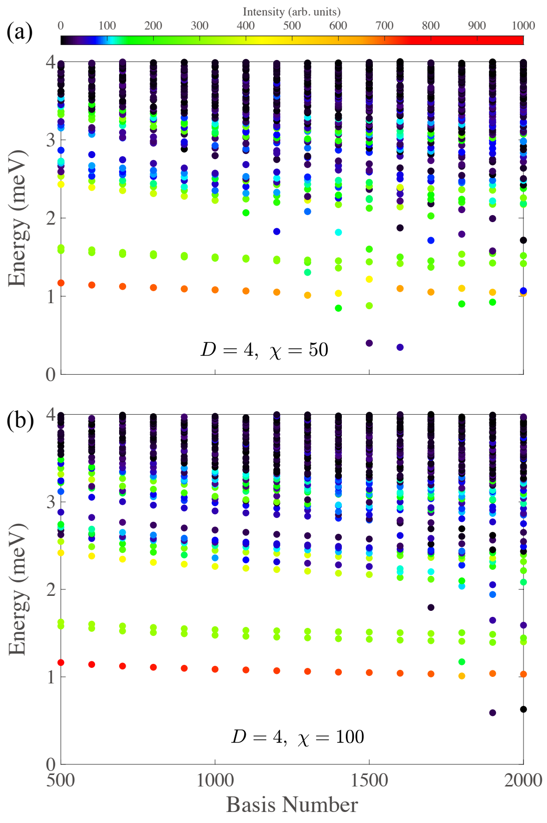


FIG. S5. Excitation spectra of the anisotropic TLAFHM ($\Delta = 0.95$) as a function of the basis number of the norm matrix for the $D = 4$ state at the $M$ point. The boundary bond dimension used by CTMRG is (a) $\chi = 50$ and (b) $\chi = 100$. The color denotes the spectral weight.

find that there is no instability in the calculation.

Figure S4 shows how the excitation spectra vary with the basis number of the norm matrix used for solving the generalized eigen-equation at the $M$ point for the $D = 2$ state. The norm matrix is calculated with high precision by utilizing a relatively large $\chi = 50$. The converged behavior of the spectra with the basis number of the norm matrix indicates that the $D = 2$ norm matrix is well-conditioned after removing all the null modes.

However, it is generally quite difficult to calculate very accurately the norm matrix by employing CTMRG or the boundary MPS when $D$ becomes larger than 2. If the norm matrix is not that accurately calculated, it may still become ill-conditioned no matter if the null modes are removed or not [R10, R11]. To remove this instability, one has to take a lower rank approximation for the norm matrix by discarding its ill-conditioned eigenvalues.

Figure S5 shows how the spectra vary with the basis number of the norm matrix retained for the $D = 4$ state at the $M$ point. The dimension of the norm matrix is about 2000 when $D = 4$. In case the boundary bond dimension $\chi = 50$, Fig. S5 (a), some spurious eigenlevels begin to appear in the excitation spectrum when the basis number is greater than 1100. Reducing the error in the norm matrix by increasing $\chi$ to 100, we find that the number of ill-conditioned eigenvalues is also dramatically reduced. In this case, the instability in the excitation spectra occurs only when the basis number becomes larger than 1700 (Fig. S5 (b)). It shows that the accuracy of the norm matrix is a vital control parameter for resolving the ill-condition problem.

Moreover, we find that the accuracy of the norm matrix evaluated with CTMRG depends strongly on the size of the unit cell in the ground state iPEPS. The smaller the unit cell, the higher the accuracy of the norm matrix if the same number of boundary basis states $\chi$ are used in the CTMRG calculations. For this reason, we adopt the iPEPS ansatz (Q1), whose size of the unit cell is 1, by grouping three inequivalent spins together.

## V. BOND DIMENSION DEPENDENCY OF SPIN EXCITATION SPECTRA

Now let us consider how fast the spin excitation spectra converge with the bond dimensions $\chi$ and $D$ for the $\Delta = 0.95$ TLAFHM.

Figure S6 shows the $D = 4$ spectral function at the $M$ point obtained by CTMRG with three different $\chi = 50, 70$ and 100 and two Lorentzian broadening parameters $\eta = 0.04$ and 0.1 meV. If a small Lorentzian broadening parameter $\eta$ is used ($\eta = 0.04$ meV, which equals $\approx 0.46$ Kelvin, lower than the measured temperature 1.7 Kelvin of the neutron scattering

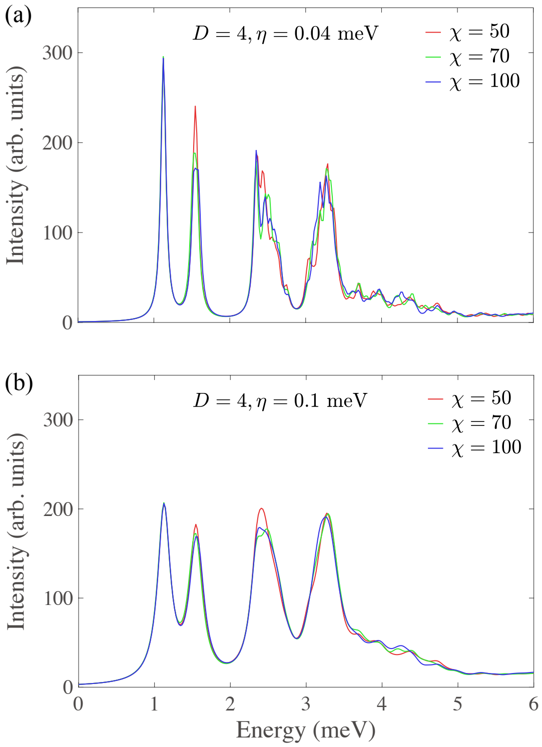


FIG. S6. Comparison of the spectral functions at M point obtained with three different $\chi = 50, 70$ and 100 and two Lorentzian broadening parameters $\eta = 0.04$ meV in (a) and 0.1 meV in (b).

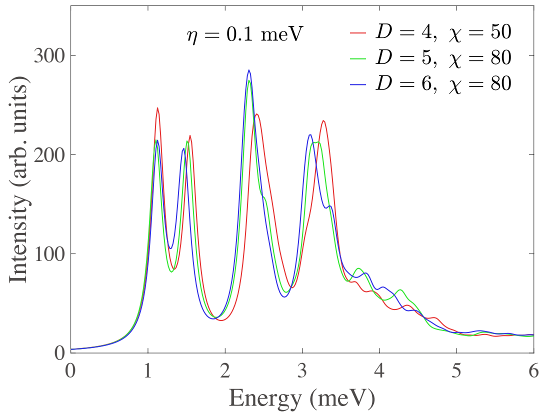


FIG. S7. Spectral functions at the M point obtained from the $D = 4, 5$ and 6 PEPS.

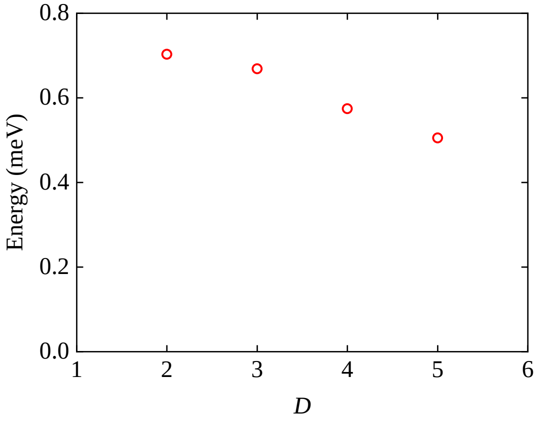


FIG. S9. Minimal spectral gap as a function of bond dimension $D$. The lowest spectral gap of the XXZ model occurs at the K point (see. Fig. S8) in the Brillouin zone. The gap values are obtained by contracting the effective Hamiltonian tensor network states of the excited states using the corner transfer matrix renormalization group method with a bond dimension $\chi = 50$ for $D = 2, 3, 4$ and $\chi = 60$ for $D = 5$.

experiment [R12]), there are small fluctuations in the high-energy peaks. On the other hand, if we set $\eta = 0.1$ meV ($\approx 1.16$ Kelvin, closer to the measurement temperature), we find that the four peaks converge quite well with the increase of $\chi$. It suggests that the energy error of our numerical results for the $D = 4$ case is roughly about 0.1 meV, higher than 0.04 meV.

Figure S7 compares the spectral functions at the M point obtained using the $D = 4, 5$ and 6 PEPS wave functions. The four-peak structures are observed in all the cases. Only the peak energies are slightly moved with the bond dimension $D$. Hence, the key features of the spin excitation spectra we obtained are intrinsic properties of TLAFHM.

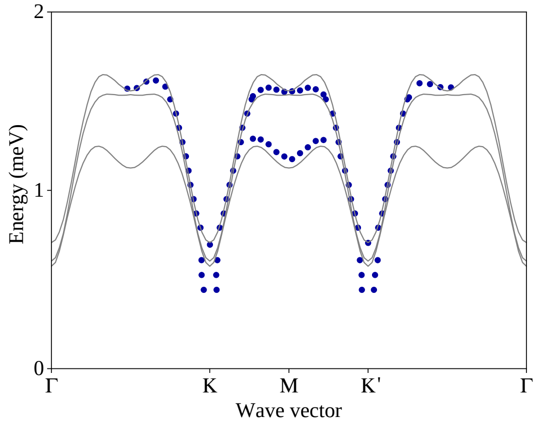


FIG. S8. Comparison of the numerical results (gray curves) of the energy dispersion relations of the three magnon bands with the experimental ones (blue dots). The experimental results are reproduced from the data published in the supplemental materials of Ref. [R12].

## VI. ENERGY DISPERSION OF THE THREE MAGNON BANDS

The lowest three excitation bands shown in Fig. 1.**c** in the main text are the three magnon bands. Fig. S8 compares the numerical results for the energy dispersion of these bands with the experimental data [R12]. Our results agree with the experimental ones, except the low-energy spectra around the K point associated with the gapless Goldstone mode. In the PEPS representations, the excitation is always gapped if $D$ is finite. The gap vanishes only in the limit $D \to \infty$. At any finite $D$, it is expected that the minimal excitation gap should decrease with the increase of $D$. This, as shown in Fig. S9, is indeed what we see in our calculation. In principle, the energy gap should converge with $D$ in certain power law for sufficiently large $D$ in a gapless system [R13]. As the values of $D$ that were used in our calculation are still very small, our data have not yet entered this power-law converged regime.

## VII. INTERACTION ANISOTROPY DEPENDENCY OF SPIN EXCITATION SPECTRA

Linear spin wave theory predicts that the spin excitation spectra of TLAFHM heavily depend on the anisotropy $\Delta$ (see Fig. S10 (d-f). In particular, the $1/S$ nonlinear spin wave theory (NLSW) [R14] suggested that the anisotropy may cause an instability in the low-energy magnon spectra due to the spontaneous two-magnon decay. In particular, NLSW predicts that the magnon decay is kinematically allowed in a large portion of the Brillouin zone when $\Delta > 0.92$, whereas this instability disappear when $\Delta < 0.92$.

For $Ba_3CoSb_2O_9$, the anisotropic parameter $\Delta$ of is about 0.95 according to experimental measurements. Hence the low-energy magnon excitations of $Ba_3CoSb_2O_9$ should be

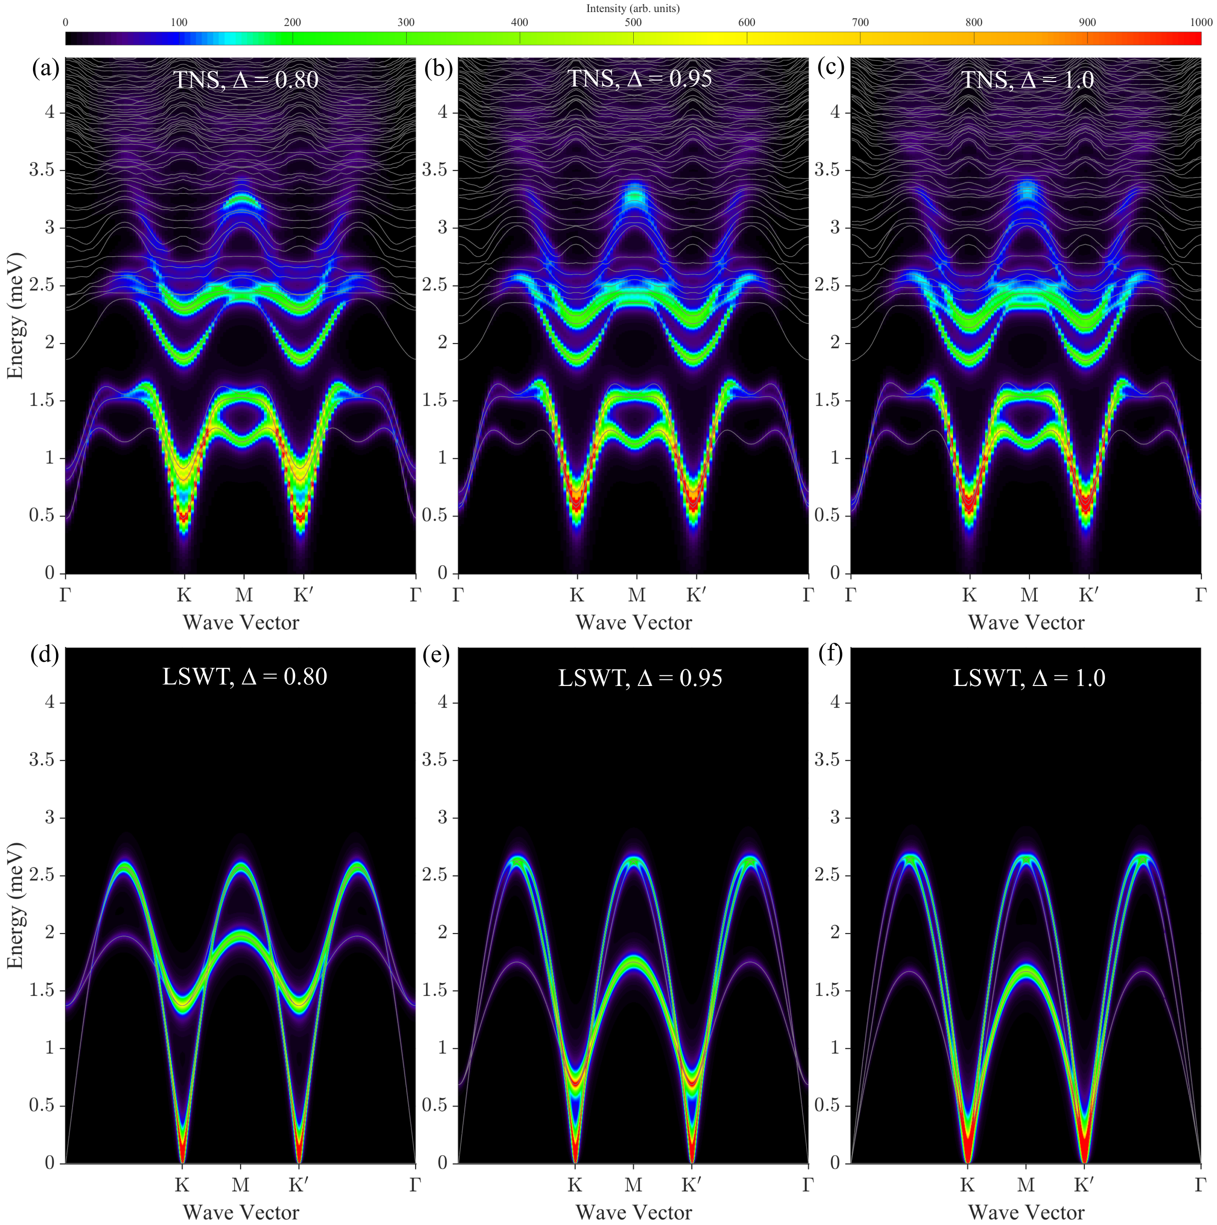


FIG. S10. Comparison of spin excitation spectra obtained using the tensor-network method (a-c) with those obtained by spin-wave theory (d-f) for TLAFHM with different anisotropic parameters $\Delta = 0.8$, $0.95$, and $1.0$, respectively.

broadened due to finite lifetime caused by the magnon decay according to NLSW. However, the neutron scattering experiments observed sharp low-energy magnon excitations. This motivates us to investigate how the spin excitation spectra vary with the anisotropy.

We calculate the spin excitation spectra for the three representative cases with $\Delta = 0.8, 0.95$ and $1.0$, respectively. Different from the prediction of NLSW, our results show sharp low-energy magnon excitations for all the three cases (Fig. S10 (a-c)). Moreover, we find that the overall spectra, including the 'W'-like high-energy excitations and low-energy roton-like excitations, only slightly depend on the anisotropic values. Thus it strongly suggests that there is not an instability caused by the two-magnon decay in the anisotropic TLAFHM with $0.8 \leq \Delta \leq 1$.

There are two main differences due to anisotropy. First, with the decrease of anisotropy, the excitation of the second and third low-energy magnons at the K point will gradually rise up, but the changes are significantly less than those predicted by the linear spin wave theory. Second, with the increase of anisotropy, the spectra at about 1.5 meV and 2.3 meV around the M point become more and more flat simultaneously, suggesting that there is a repulsive interaction between the high- and low-energy excitations. This is consistent with the picture of the avoided magnon decay due to level-continuum repulsion proposed in Ref. [R15].

[R1] H.-J. Liao, J.-G. Liu, L. Wang, and T. Xiang, Phys. Rev. X **9**, 31041 (2019).
[R2] Y. Iqbal, W.J. Hu, R. Thomale, D. Poilblanc, and F. Becca, Phys. Rev. B **93**, 144411 (2016).
[R3] O. Götze, J. Richter, R. Zinke, and D. J. J. Farnell, J. Magn. Magn. Mater. **397**, 333 (2016).
[R4] D. Heidarian, S. Sorella, and F. Becca, Phys. Rev. B **80**, 012404 (2009).
[R5] L. Capriotti, A. E. Trumper, and S. Sorella, Phys. Rev. Lett. **82**, 3899 (1999).
[R6] R. P. Feynman, Phys. Rev. **94**, 262 (1954).
[R7] S.Östlund and S. Rommer, Phys. Rev. Lett. **75**, 3537 (1995).
[R8] J. Haegeman, B. Pirvu, D. J. Weir, J. I. Cirac, T. J. Osborne, H. Verschelde, and F. Verstraete, Phys. Rev. B **85**, 100408 (2012).
[R9] L. Vanderstraeten, M. Mariën, F. Verstraete, and J. Haegeman, Phys. Rev. B **92**, 201111 (2015).
[R10] L. Vanderstraeten, J. Haegeman and F. Verstraete, Phys. Rev. B **99**, 165121 (2019).
[R11] B. Ponsioen, F. F. Assaad, and P. Corboz, SciPost Phys. **12**, 6 (2022).
[R12] D. Macdougal, S. Williams, D. Prabhakaran, R. I. Bewley, D. J. Voneshen, and R. Coldea, Phys. Rev. B **102**, 064421 (2020).
[R13] H. J. Liao, Z. Y. Xie, J. Chen, Z. Y. Liu, H. D. Xie, R. Z. Huang, B. Normand, and T. Xiang, Phys. Rev. Lett. **118**, 137202 (2017)
[R14] A. L. Chernyshev and M. E. Zhitomirsky, Phys. Rev. Lett. **97**, 207202 (2006).
[R15] R. Verresen, R. Moessner, and F. Pollmann, Nat. Phys. **15**, 750 (2019).
